# Supplementary material for: Federated Unbiased Learning to Rank
Source: arXiv:2105.04761 source file (2021-05-11)
Supplement: Supplementary file 1 [file appendix.tex]

%!TEX root = paper.tex
\onecolumn
\section{$\fedopt$}
We present $\fedopt$ in~\cref{alg:fedopt} for convenience. 

\begin{algorithm}[tb]
	\caption{$\fedopt$ (Algorithm 1 in \cite{reddi2020adaptive})}
	\label{alg:fedopt}
	\begin{algorithmic}[1]
		\Input  $\mathbf{w}_0$, $\sf ClientOpt$ and $\sf ServerOpt$
		\For{$t = 0, \ldots $}
		\State \label{alg: sample broadcast} Sample a client subset $\cU$  and broadcast $\mathbf{w}_{t}$ 
		\For{$u \in \cU$}
		\Comment{In parallel}
		\State 	  $\vw^*_{t, u} \leftarrow \sf{ClientOpt} (\cE_u,\vw_t, \ell_l, t)$
		\State $\Delta_{t, u} =\vw^*_{t, u}-\vw_{t}$
		\EndFor
		\State $\Delta_{t}= \frac{1}{|\cU|} \sum_{u \in\cU} \Delta_{t, u} $ \Comment{Server side}
		\State $\vw_{t+1} = {\sf ServerOpt}(\vw_{t}, \Delta_t, t)$
		\EndFor
	\end{algorithmic}
\end{algorithm}

\section{Additional Experimental Results}
%!TEX root = paper.tex

\begin{figure*}[t]
	\centering
	\includegraphics{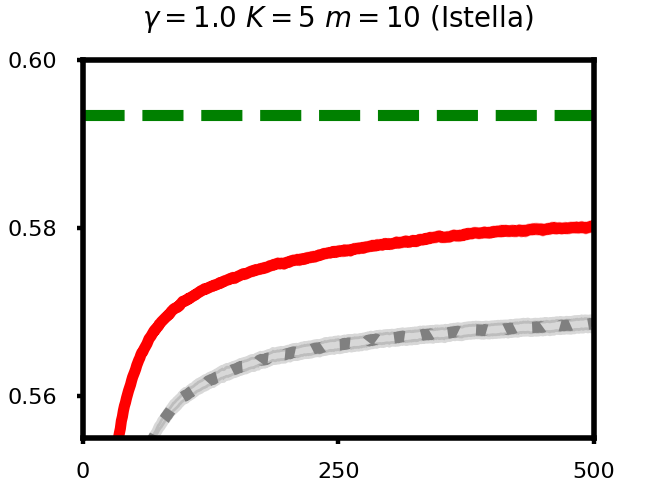}
	\includegraphics{istellas-var1-gammamean1.0npos10nclickperuser10.png}
	\includegraphics{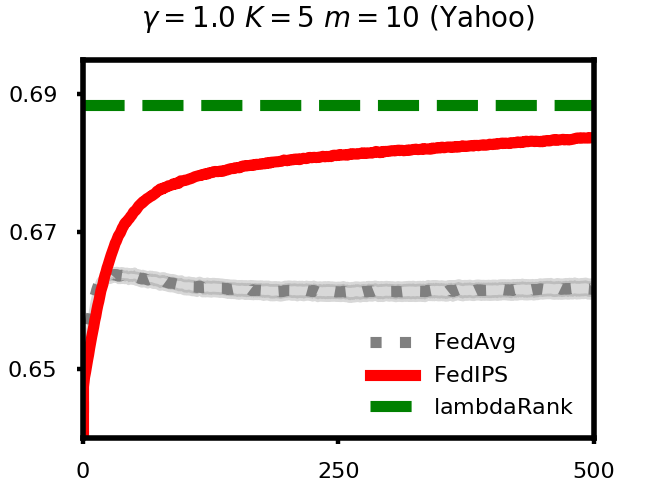}
	\includegraphics{set1-var1-gammamean1.0npos10nclickperuser10.png}
	\caption{NDCG@$5$ of $\fedips$ (red solid line), $\fedavg$ (gray dotted line) and $\lambdalinear$ (green dashed line). The x-axis indicates the number of round. $K$ is the number of positions and $m$ is the number of clicks per user. Results are averaged over $30$ repeats. Shaded areas are the standard errors of  estimates.}
	\label{fig: performance}
\end{figure*}

\begin{figure*}
	\centering
	\includegraphics{bias-istellas-1-gammamean0.5npos5nclickperuser10}
	\includegraphics{bias-istellas-1-gammamean1.0npos5nclickperuser10}
	\includegraphics{bias-istellas-1-gammamean1.5npos5nclickperuser10}
	\includegraphics{bias-istellas-1-gammamean2.0npos5nclickperuser10}	
	\includegraphics{bias-set1-1-gammamean0.5npos5nclickperuser10}
	\includegraphics{bias-set1-1-gammamean1.0npos5nclickperuser10}
	\includegraphics{bias-set1-1-gammamean1.5npos5nclickperuser10}
	\includegraphics{bias-set1-1-gammamean2.0npos5nclickperuser10}	
	\caption{Impact of  different levels of noise $\gamma$ on the performance (NDCG@$5$) of $\fedips$ (red solid line) and $\fedavg$ (gray dotted line) with $K=5, m=10$. 
		The green dashed lines are results of $\lambdalinear$ that is trained in an offline full-information manner. 
		The x-axis indicates the number of round.  }
	\label{fig: bias}
\end{figure*}

\section{Experimental results}
\label{sec: experimental results}

We report our experimental results. 
In \cref{sec: effective of ips}, we report the effectiveness of IPS and answer the question of how does the proposed  $\fedips$ compare to $\fedavg$ as well as the full-information baseline $\lambdalinear$. 
Then, we study impacts of position bias, numbers of clients and  number of clicks on the performance in \cref{sec: severtiy of bias,sec: number of devices,sec: impact of number of clicks}, respectively.
Finally, in \cref{sec: ips estimation}, we show some inspirations on how to estimate the personalized IPS in \ac{FL}.

\subsection{Effectiveness of IPS}
\label{sec: effective of ips}

We first assess the general performance of $\fedips$ and baselines. 
We use NDCG@$5$ as the evaluation metric. 
We report the performance of $\fedips$ and $\fedavg$ on both Istella and Yahoo datasets in \cref{fig: performance}.
We choose $\gamma=1.0$ as the standing example. 
Each round, we simulate $2000$ clients and each client issues $10$ clicks. 
We update the algorithms with $2000 \times 10 = 20000$ clicks and we run the experiments for $500$ rounds. 
Thus, in total, there are $1$ million clicks. 
On both datasets, $\fedips$ outperforms $\fedavg$ with large gaps, and the gaps on the Yahoo dataset are larger than that on the Istella dataset. 
This is because the Istella dataset is a slightly harder one comparing to the Yahoo dataset since the former one contains more documents per query and most of them are irrelevant. 
We also observe that, on the Yahoo dataset, the gray lines ($\fedavg$) stop growing while the red lines ($\fedips$) are still climbing after $500$ iterations. 
Comparing to the $\lambdalinear$, on both datasets, we observe that there are still gaps between $\fedips$ and $\lambdalinear$.
However, on the Yahoo datasets, $\fedips$ is approaching  $\lambdalinear$.  
We emphasize that $\lambdalinear$ enjoys two additional benefits from its offline full-information learning setup: 
\begin{enumerate*}
	\item $\lambdalinear$ learns from the whole query-document pairs, and the IID assumption holds. 
	\item $\lambdalinear$ learns from real relevance labels, which are noise and bias free. 
\end{enumerate*}

After all, the results indicate that $\fedips$ outperforms $\fedavg$ in the task of federated unbiased \ac{LTR}, and comparing to the full-information $\lambdalinear$, there is still room for improvement. 
In the following experiments, we analyze the impact of different factors of \ac{FL} on learning algorithms.
%As $\lambdalinear$ is not affected by factors, we omit it in the rest of experiments.

\subsection{Severity of Bias}
\label{sec: severtiy of bias}
Then, we study the impact of position bias on the performance. 
We choose $K=5$ and $m=10$ as the standing example. 
We assess $\fedips$ and $\fedavg$ with $\gamma \in \{0.5,  1.0, 1.5, 2.0\}$ and  report the results of $\fedips$ and $\fedavg$ on both datasets in \cref{fig: bias}. 
The larger $\gamma$ indicates the more severe position bias. 
\cref{fig: bias} shows that the performance of $\fedavg$ is heavily impacted by the position bias, and the performance drops dramatically when the severity of bias increases.
As for the proposed $\fedips$, we observe that the position bias does not have a heavy impact on the performance on the Yahoo dataset. 
Although $\fedips$ performs the best in the case of $\gamma=0.5$, drops in the performance are small among different values of $\gamma$. 
On the Istella dataset, we see a slightly different behavior of $\fedips$. 
There is a clear drop in the performance of $\fedips$ from $\gamma=0.5$ to $\gamma=1.0$,  and the performance  contains larger variances when $\gamma$ becomes larger. 
We believe that  this is because the Istella dataset is a slightly harder one than the Yahoo dataset. 
After all, these results confirm that the proposed $\fedips$ can handle the position bias in the click feedback.

\begin{figure}[t]
	\centering
	\includegraphics{device-istellas-1-10}
	\includegraphics{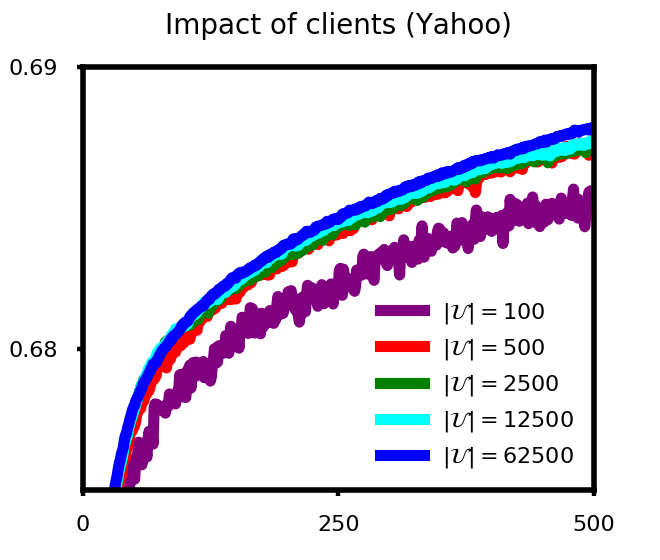}
	\caption{ 	Impact of the number of clients per round on the performance (NDCG@$5$)  of $\fedips$ with $K=5, m=10, \gamma=1.0$. The x-axis indicates the number of round. }
	\label{fig: devices}
\end{figure}

\subsection{Impact of number of clients}
\label{sec: number of devices}
In \ac{FL}, it is easier to collect a large number of clients with few clicks than a relatively small number of clients with many clicks~\citep{mcmahan2017learning}. 
More clients involved per round enables us to get a more accurate estimator on the global gradient. 
In this section, we study the impact of different numbers of clients on the performance of $\fedips$, and answer the question: to what extend does a larger number of clients help to increase the performance of $\fedips$. 
We choose the number of clients as follows: $|\cU| \in \{100, 500, 2500, 12500, 62500 \}$. 
The results on both datasets are displayed in \cref{fig: devices}. 
To our surprise, we find that after $|\cU|$ reaches to a level, e.g., $|\cU| = 2500$ for both datasets, increasing $|\cU|$ does not improve the performance of $\fedips$ a lot. 
Particularly, $\fedips$ with $|\cU|=100$ falls behind other and the learning curves have large fluctuations. 
We notice the similar fluctuation for $\fedips$ with $|\cU|=500$. 
This is because, with few clients, the estimated global gradient is noisy. 
We also observe that, when $|\cU| \geq 2500$, $\fedips$  does not benefit too much from by including more clients. 
This observation is from the fact that after including enough clients per round, $\fedips$ estimates rather accurate global gradients, and thus, the variance in the estimator is not the bottleneck of $\fedips$.

As a summary, the number of clients has an impact on the variance of the estimated gradient. 
The performance of $\fedips$ can be improved by including more clients per round.
However, after a certain number of clients, when the estimated gradient has little variance, $\fedips$ no longer benefit much from including more clients. 

\subsection{Impact of number of clicks}
\label{sec: impact of number of clicks}
The IPS-based methods generally have large variances.
To reduce the variance, one way is to increase the size of training data. 
In our federated setup, the training data are from user interactions, i.e., clicks. 
In this section, we study the impact of clicks per round on the performance of $\fedips$. 
We choose $m \in \{5, 10, 20, 30, 50\}$.  
$m \in \{20, 30, 50\}$ are less realistic setups, but we want to check the optimal performance of $\fedips$. 
The results on the Yahoo and Istella datasets are reported in \cref{fig: clicks}. 
Generally, we observe the trend that performance of $\fedips$ goes up when the number of clicks goes up. 
However, we also notice that after a certain number of clicks, e.g., $m=20$ for the Yahoo dataset and $m=30$ for the Istella dataset, the gaps of $\fedips$ with different $m$ are small. 
This observation is caused by the similar reason as discussed above. 
After a certain $m$, $\fedips$ estimates an accurate local gradient and the bottle neck of the performance of $\fedips$ does not come from the variance.

\begin{figure}[t]
	\centering
	\includegraphics{clicks-istellas-1-estimated0}
	\includegraphics{clicks-set1-1-estimated0}
	\caption{
		Impact of the number of clicks $m$ on the performance (NDCG@$5$) of $\fedips$ with $K=5, \gamma=1.0$. The x-axis indicates the number of round. }
	\label{fig: clicks}
\end{figure}

\subsection{Effectiveness of estimated IPS}
\label{sec: ips estimation}
In previous experiments, we assume that the propensity score is known. 
This is a valid assumption, since the propensity score can be estimated from the controlled online experiments~\citep{joachims2017unbiased} or estimated from the click logs~\citep{wang2018position}. 
As for the \ac{FL} setup, the click logs are located in local clients, the amounts of which are typical small, e.g., $5$ or $10$ in our experiments. 
Two natural questions are how to estimate IPS in \ac{FL},  and whether $\fedips$ with the estimated propensity outperforms $\fedavg$. 

To estimate the propensity score, we follow the approach proposed by \citet{wang2018position}, where the propensity score is estimated in a regression-based EM method. 
Particularly, a function $F$ is used to estimate the hidden variable $r_{q,d}$. 
The nice part of this approach is that the function $F$ can be shared across all clients and optimized in a \ac{FL} way. 
In this experiment, we choose a linear function $F(\vx; \mu)$ to estimate the relevance score, which is updated in a \ac{FL} manner.  
We estimate the personalized IPS, and run a slightly different version of Algorithm~1 in~\citep{wang2018position} on each local client $s$.
The differences are that we do not reset $F(\vx; \mu)$ before the iteration, and the output of the algorithm is the local update of $F_s(\vx; \mu)$. 
On the server side, the local updates are averaged to obtain the ``pseudo gradient'', which is  then used to update $F(\vx; \mu)$. 

Generally, we expect that more clicks per round lead to a more accurate estimator of propensity score. 
Thus, we conduct this experiments with different numbers of clicks and  report the results of $\fedips$ with the estimated propensity score in \cref{fig: clicks estimated}.  
We observe that $\fedips$ with the estimated IPS outperforms the biased $\fedavg$ on both datasets. 
Among all cases, $m=5$ is the hardest one, because some positions do not receive any click per round, and the estimated IPS is rather noisy. 
This can also be observed in our results.
$\fedips$ with $m=5$ performs closely to $\fedavg$ on the Istella dataset. 
On the Yahoo dataset, $\fedips$ loses to $\fedavg$ at the  beginning and only comes back after $100$ rounds. 
Meanwhile, there are gaps between the performance of $\fedips$ with the estimated IPS and the real IPS (comparing to results in \cref{fig: clicks}). 
As a summary, $\fedips$ with the estimated propensity score outperforms $\fedavg$.
However, there are still some spaces for the improvement.

\begin{figure}[t]
	\centering
	\includegraphics{clicks-istellas-1-estimated1}
	\includegraphics{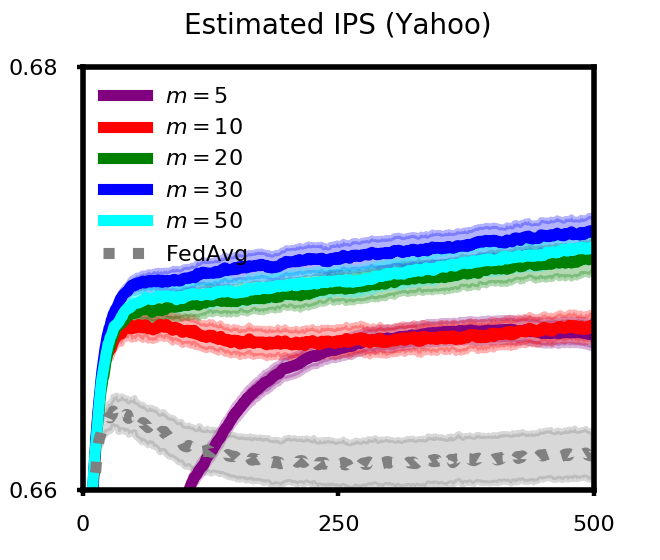}
	\caption{Performance (NDCG@$5$)  of $\fedips$ with the estimated IPS with different numbers of clicks $m$, where $\gamma = 1.0$ $K=5$. The x-axis indicates the number of round. }
	\label{fig: clicks estimated}
\end{figure}
